# Supplementary material for: Topological Approximate Dynamic Programming under Temporal Logic Constraints
Source: arXiv:1907.10510 source file (2019-09-26)
Supplement: Supplementary file 1 [file appendix.tex]

\begin{algorithm}[!htb]
	\SetKwInOut{Input}{Input}
	\SetKwInOut{Output}{Output}
	\Input{an MDP $M= \langle \calS, \calA, P, R \rangle$, $\delta:$ the threshold value}
	initialize $V$ arbitrarily\;
	\While{true}{
		$Bellman\_error \leftarrow 0$\;
		\For{each state $s \in \calS$}{
			$oldV \leftarrow V(s)$\;
			$V(s)\leftarrow \min_{a\in \calA(s)} [R(s,a) + \sum_{s' \in S} P(s' \mid s, a) V(s')]$\;
			$Bellman\_residual(s) \leftarrow |V(s)- oldV|$\;
			$Bellman\_error \leftarrow \max{(Bellman\_error, Bellman\_residual(s))}$
			}\If{$Bellman\_error < \delta$}
		{\KwRet{$V$}}
	}
	\caption{(Gauss-Seidel) Value Iteration}
	\label{alg:VI}
\end{algorithm}

\subsection{Probabilistic Automaton}
The \ac{pa} may be defined as an extension of a \ac{nfa} $(Q,\Sigma,\delta, q_0,F)$, together with two probabilities: the probability $P$ of a particular state transitions taking place, and with initial state $q_0$ replaced by a stochastic vector giving the probability of the automation being in a given initial state.
For the ordinary non-deterministic finite automaton, one has
\begin{itemize}
	\item a finite set of states $Q$
	\item a finite set of input symbols $\Sigma$
	\item a transition function $\delta: Q \times \Sigma \rightarrow P(Q)$
	\item a set of states $F$ distinguished as accepting (or final) states $F \subset Q$
\end{itemize}
Here, $P(Q)$ denotes the power set of $Q$.
A Rabin automaton is one for which the initial distribution $v$ is a coordinate vector; that is, has zero for all but one entries, and the remaining entry being one.

The set of Languages recognized by \ac{pa} are called stochastic languages. They include the regular languages as a subset.

In this case, a \ac{pa} is considered, which is an example to prove the correctness of the implementation of the algorithm~\ref{alg:TVI}. The automaton is shown in Fig.~\ref{fig:automaton}. Note that in the automaton figure, the transition: $P(q,a,q)=1$ is not drawn for the purpose of simplicity.
\\
For a \ac{nfa}, $Q = \{a,b,c,d,e,f,g,h\}$,$\Sigma = \{A,B\}$, $F = \{d\}$, and the corresponding transition probability is shown in the figure~\ref{fig:automaton}
\begin{figure}[htbp]
	\centering
	\begin{tikzpicture}[->,>=stealth',shorten >=1pt,auto,node distance=3cm,scale=0.75,semithick, transform shape]
		\tikzstyle{every state}=[fill=black!10!white]
		\node[initial,state]    (a)                    {$a$};
		\node[state]            (b) [right of=a]       {$b$};
		\node[state]            (c) [right of=b]       {$c$};
		\node[state, accepting] (d) [right of=c]       {$d$};
		\node[state]            (e) [below of=a]       {$e$};
		\node[state]            (f) [right of=e]       {$f$};
		\node[state]            (g) [right of=f]       {$g$};
		\node[state]            (h) [right of=g]       {$h$};
		\path[->]   (a) edge[loop above]            node            {$A: 0.1$}  (a)
		edge                        node            {$A: 0.9$}  (b)
		edge                        node            {$B: 1.0$}  (f)
		                        
		(b) edge[loop above]            node[below]     {$A: 0.5$}  (b)
		edge                        node            {$A: 0.5$}  (c)
		edge                        node            {$B: 0.5$}  (f)
		edge[in=195,out=255,loop]   node[above]     {$B: 0.5$}  (b)
		                        
		(c) edge                        node            {$A: 0.8$}  (d)
		edge[loop above]            node            {$A: 0.2$}  (c)
		edge                        node[left]      {$B: 0.1$}  (g)
		edge[in=195,out=255,loop]   node            {$B: 0.9$}  (c)
		                        
		(e) edge                        node            {$A: 0.4$}  (a)
		edge[loop below]            node            {$A: 0.6$}  (e)
		                        
		(f) edge                        node            {$A: 0.7$}  (e)
		edge[in=15,out=75,loop]     node            {$A: 0.3$}  (f)
		edge                        node            {$B: 0.8$}  (g)
		edge[loop below]            node            {$B: 0.2$}  (f)
		                        
		(g) edge[bend right]            node[right]     {$A: 0.1$}  (c)
		edge[loop below]            node            {$A: 0.9$}  (g)
		(h) edge                        node            {$A: 0.4$}  (g)
		edge[loop above]            node            {$A: 0.6$}  (h)
		;
	\end{tikzpicture}
	\caption{\ac{pa}}
	\label{fig:automaton}
\end{figure}
\begin{figure}[!htb]
	\centering
	\includegraphics[width=\linewidth]{division.png}
	\caption{Partition of the Probabilistic Automaton}
	\label{fig:partition}
\end{figure}
After applying the Kosaraju's algorithm, a partition of the automaton is acquired plotted in Fig.~\ref{fig:partition}, \ie $\{id[\{a,b,e,f\}] = 3,id[\{c,g\}]=2,id[\{d\}]=1,id[\{h\}]=1\}$, where the number is the corresponding topological order.

We use algorithm~\ref{alg:VI} to update the values of each \ac{scc} according to the topological order until the error is smaller than the threshold $\delta$. Note that in our case we set the $\delta = 1e-8$ for both algorithm including \ac{tvi} and Softmax Value Iteration. 

The comparison of solution of the \ac{tvi} and the ground truth computed by Softmax Value Iteration is the following:
\begin{table}[!htb]
	\centering
	\resizebox{\linewidth}{!}{%
		\begin{tabular}{|c|c|c|}
			\hline
			State & Topological Value Iteration & Softmax Value Iteration \\ \hline
			2     & 16.07216154780488           & 16.072161547858556      \\ \hline
			4     & 0.0                         & 0.0                     \\ \hline
			6     & 11.053384709181309          & 11.053384714971298      \\ \hline
			5     & 11.98721221624176           & 11.987212229750455      \\ \hline
			3     & 19.59670519292653           & 19.59670519290457       \\ \hline
			8     & 9.878620261212003           & 9.878620263524176       \\ \hline
			1     & 14.319954261575155          & 14.319954261548876      \\ \hline
			7     & 11.328771513013372          & 11.328771518035124      \\ \hline
		\end{tabular}%
	}
	\caption{Comparison between Topological Value Iteration and Softmax Value Iteration}
	\label{table:comparision}
\end{table}
From the Table~\ref{table:comparision}, we can see that the \ac{tvi} achieves tight error bound, which proves the correctness of the implementation.
\\To compare the complexity of \ac{tvi} and Softmax Value Iteration, both \ac{cpu} time is recorded, the elapsed time of both algorithms is $0.0169 s$ and $0.0199 s$ respectively. Moreover, to show that the times of total Bellman Backup Operations can be reduced due to the partition and update based on the Topological order, the total times of Bellman Backup Operations are counted. For the \ac{tvi}, for different \ac{scc}, the Softmax Value Iteration converges after $1, 222, 196, 50$ with respect to topological order of the \ac{scc}s. So the total number of the Bellman Backup Operations for the \ac{tvi} is 469. On the other side, the total number of Bellman Backup Operations using the Softmax Value Iteration for the entire \ac{mdp} is 888. The total amount of Bellman Backup Operations is reduced around $47\%$. The reason that in term of the \ac{cpu} time there is no big difference, like the time is reduced by $15\%$ may caused by passing parameters between functions. But it is safe to say that for bigger \ac{mdp}, the difference between time should be much bigger.

\paragraph*{Greedy policy Graph} The basic heuristic search is to expand an action only when necessary, and leads to a more conservative backup strategy. This strategy helps save a lot of unnecessary backups.
Heuristic search algorithms have two main features:
\begin{itemize}
	\item Values of the state space are initialized by an admissible and consistent heuristic function.
	\item The search is limited to states that are reachable from the initial state.
\end{itemize}
Given the heuristic value, heuristic search generates a running \textit{greedy policy} - the best policy by one-step lookahead given the current value function, as well as the \textit{greedy policy graph} - a subset of the labelled \ac{mdp} that contains all states that are reachable from the initial state through the current greedy policy and corresponding transitions. 

A search typically starts from the initial state, and expands along a greedy action, either deterministically or stochastically. Visited states have their values back-up during the search.

\begin{theorem}
	[Action Elimination~\cite{bertsekas2007dynamic}] If a lower (resp. upper) bound of $Q^{\ast}(s, a)$ is greater (resp. lower) than an upper (resp. lower) bound of $V^{\ast}(s)$ then action $a$ cannot be an optimal action for state $s$.
\end{theorem}

\begin{algorithm}[!htb]
	\SetKwData{cpntnum}{cpntnum}
	\SetKwData{id}{id}
	\SetKwFunction{SCC}{SCC}
	\SetKwFunction{Search}{Search}
	\SetKwFunction{Product}{Product}
	\SetKwFunction{Backup}{Back-up}
	\SetKwFunction{Setreward}{Set-reward}
	\SetKwFunction{ADP}{ADP}
	\SetKwInOut{Input}{Input}
	\SetKwInOut{Output}{Output}
	\SetKw{Break}{break}
		
	\Input{a \ac{dfa} $\calA_{\varphi} = \langle \calQ, \Sigma, \delta, q_0, F \rangle$, a labeled \ac{mdp} $M = \langle S,A, \mu_0,P,\calAP, L \rangle$, $\epsilon:$ the threshold value}
% 	\{step 1: search\}\;
% 	\While{True}{
% 		$old\_value \leftarrow V_u(q_0)$\;
% 		\For{$ iter \leftarrow$ 1 \text{to} m}
% 		{
% 			$Bellman\_error \leftarrow 0$ \;
% 			\For{every state $q$}{
% 				make every state as unvisited\;}
% 			$q \leftarrow q_0$ \;
% 			\Search{$q$}\;
% 			\If{$Bellman\_error < \epsilon$}{
% 				\KwRet{$V_u$}\;}
% 		}
% 		\If{$V_{u}(q_0) / old\_value  > (100 - y)\%$}{\Break\;}
% 	}
% 	\{step 2: computation\}\;
	\{\cpntnum, \id\} $\leftarrow$ \SCC{$\calA_{\varphi}$}\;
	\For{$i\leftarrow 1$ \KwTo \cpntnum}{
		$X_i \leftarrow$ the set of states $q$ where $\id[q]= i$\;
		$\calA_{\varphi}' \leftarrow \langle X_i,\Sigma, \delta,q_0,F  \rangle$\;
		$\calM \leftarrow$ \Product{$\calA_{\varphi}', M$}\;
		\If{$i > 1$}{
			$\calM$ = \Setreward{$V$, $\calM$}}
		$V$ = \ADP{$\calM$}\;}
	\KwRet{}\;
		
	\SetKwProg{Fn}{Function}{:}{}
	\Fn{\SCC{$\calA_{\varphi}$}}{
		construct $G_R$ of $\calA_{\varphi}$\;
		construct a graph $G'_R$ which reverses the head and tail vertices of every edge in $G_R$\;
		\{call Kosaraju's algorithm \cite{cormen2009introduction}. It inputs $G_R$ and $G'_R$ and outputs \cpntnum, the total number of \ac{sccs}, and $\id: \calQ \rightarrow [1, \cpntnum]$, the id of the \ac{sccs} each state belong to, by topological order.\}\;
		\KwRet{\{\cpntnum, \id\}}\;
	}
		
% 	\SetKwProg{Fn}{Function}{:}{}
% 	\Fn{\Search{$q$}}{
% 		\If{$q \notin F$}{
% 			mark $q$ as visited\;
% 			$a \leftarrow \underset{a}{\argmax} Q(q, a)$\;
% 			\For{every unvisited successor $q'$ of action $a$}{
% 				\Search{$q'$}\;}
% 			$Bellman\_error \leftarrow \max (Bellman\_error,$ \Backup{$q$}$)$
% 		}
% 		\KwRet{}\;
% 	}
		
% 	\SetKwProg{Fn}{Function}{:}{}
% 	\Fn{\Backup{$q$}}{
% 		\For{each action $a$}{
% 			$Q(q, a) \leftarrow R(q, a) + \sum P(q' \mid q, a)V_{u}(q')$\;
% 			\If{$Q(q, a) < V_l(q)$}{
% 				eliminate $a$ from $\fq(q)$}
% 			\KwRet{}\;
% 		}
			
% 		$oldV_u \leftarrow V_u(q)$\;
% 		$V_u(q) \leftarrow \underset{a \in \fq(q)}{\max}Q(q, a)$\;
% 		$V_l(q) \leftarrow \underset{a \in \fq(q)}{\max}R(q, a) + \sum P(q' \mid q, a)V_l(q')$\;
% 		\KwRet{$|V_u(q) - oldV_u|$}
% 	}
	\caption{Topological Approximate Dynamic Programming}
	\label{alg:FTADP}
\end{algorithm}

\subsection{Linear Temporal Logic}
\ac{ltl} was developed as an expressive mean for formal reasoning about the system. 
\begin{definition}[Linear Temporal Logic~\cite{gerth1995simple}]
\ac{ltl} are constructed from a set of \ac{ap} $\calAP$, the standard Boolean operators, and the temporal operators $\Next$ and $\Until$. Precisely, the set of $\ac{ltl}$ formulas is defined inductively as follows:
\begin{itemize}
    \item if $p \in \calAP$, then $p$ is a formula,
    \item if $\varphi$ and $\psi$ are formulas, then so are $\lnot \varphi, \varphi \wedge \psi, \varphi \vee \psi, \Next \varphi$ and $\varphi \Until \psi$.
\end{itemize}
\end{definition}

Given an infinite world $w = r_0 r_1 \cdots$ over alphabet $2^{\calAP}$, we say $w$ satisfies an \ac{ltl} $\varphi$ when $w \models \varphi$. Essentially, an \ac{ltl} formula is satisfied by an infinite sequence of truth evaluations variables in $\calAP$.
The semantics of \ac{ltl} is the following.
\begin{itemize}
    \item $w \models p$ if $p \in r_0$, for $p\in \calAP$,
    \item $w \models \lnot \varphi$ if not $w \models \varphi$,
    \item $w \models \varphi \wedge \psi $ if $w \models \varphi$ and $w \models \psi$,
    \item $w \models \varphi \vee \psi $ if $w \models \varphi$ or $w \models \psi$,
    \item $w \models \Next \varphi$ if not $w_1 \models \varphi$,
    \item $w \models \varphi \Until \psi$ if there is an $i \geq 0$ such that $w_{i} \models \psi$ and $w_j \models \varphi$ for all $0 \leq j < i$
\end{itemize}
